# Supplementary material for: How to Understand Named Entities: Using Common Sense for News Captioning
Source: arXiv:2403.06520 source file (2024-03-11)
Supplement: Supplementary file 1 [file fig_common_sense.tex]

\begin{figure}
	\centering{\includegraphics[width=1.0\columnwidth]{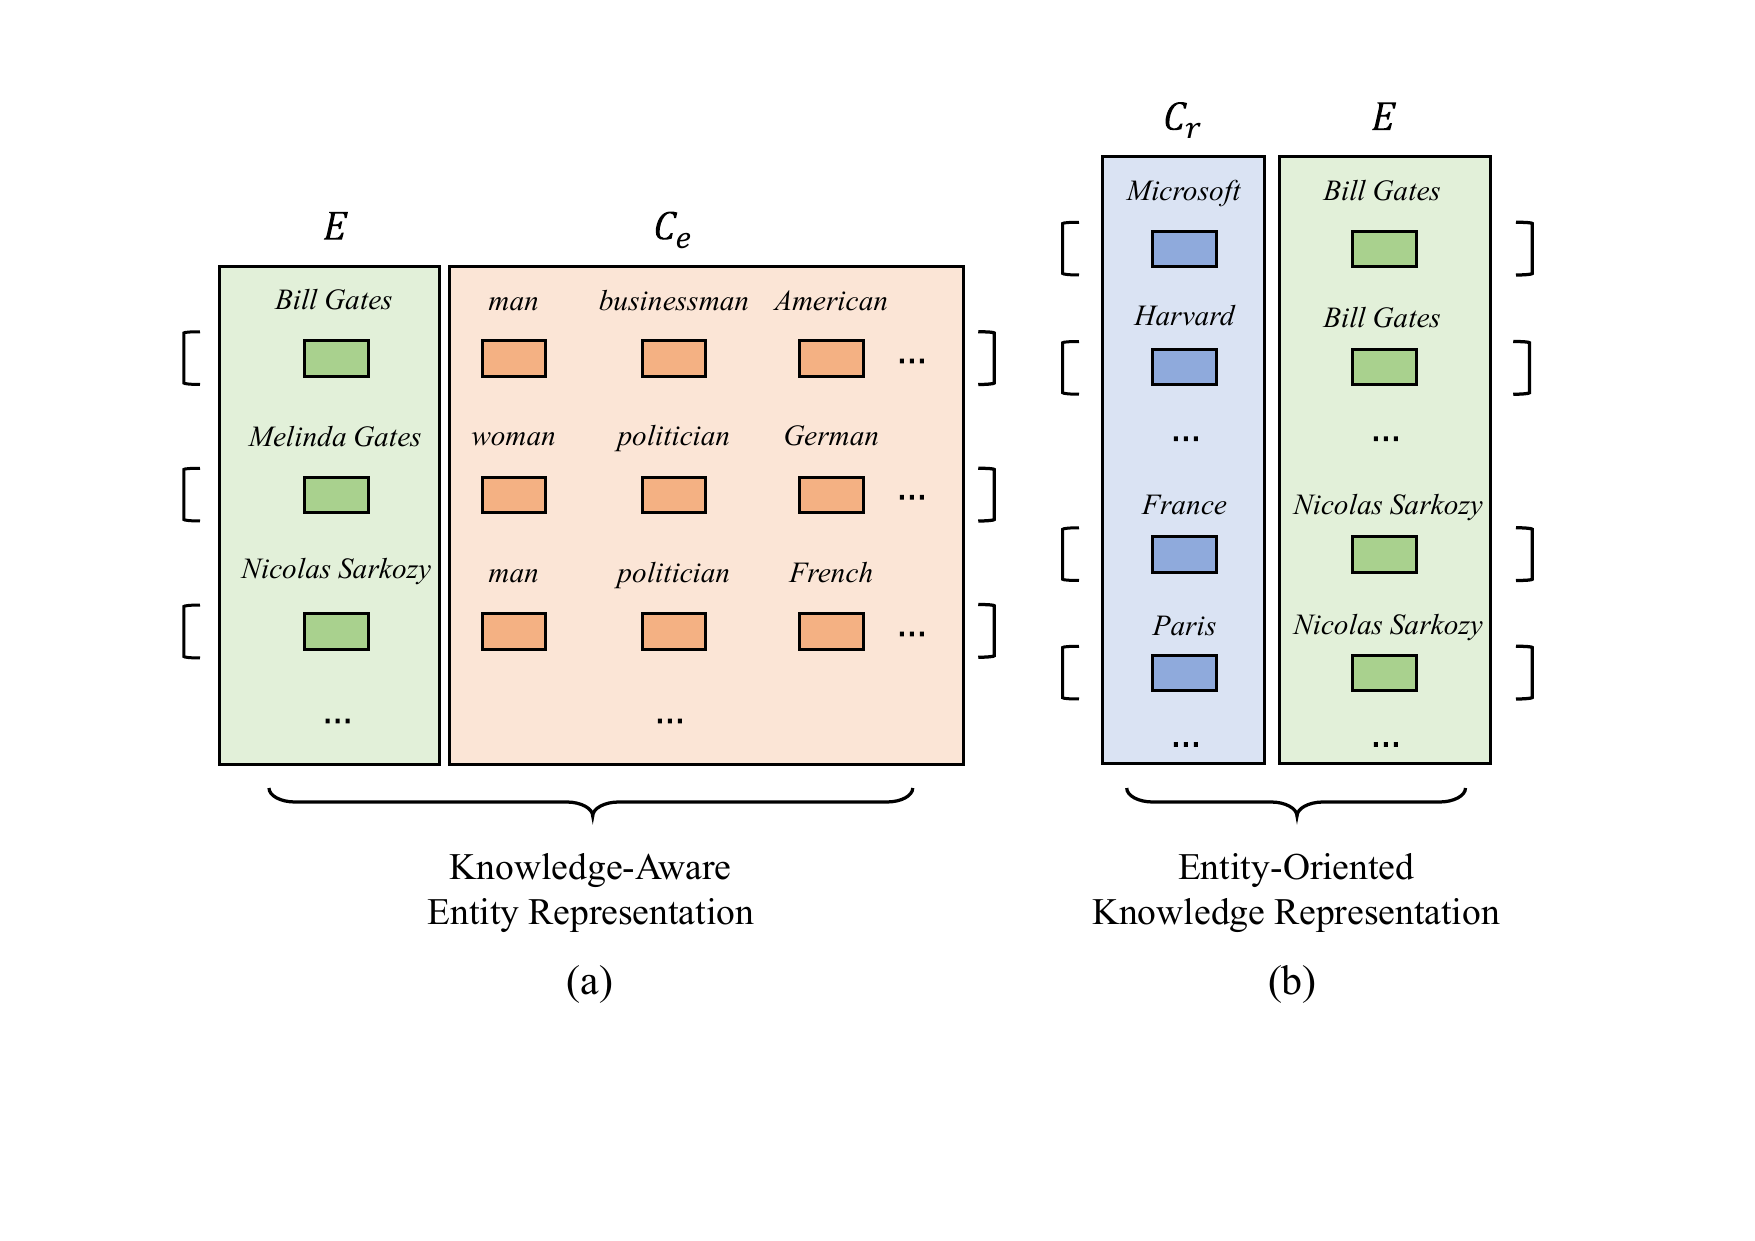}}
	\caption{
		Illustration of a) Knowledge-Aware Entity Representation in Distinguish Module (Sec. \ref{sec:distinguish} ) 
		and b) Entity-Oriented Knowledge Representation in Enrich Module (Sec. \ref{sec:enrich}) (Best viewed in color).
		}
	\label{fig:framework}
%	\vspace{-0.4cm}
\end{figure}
