# Supplementary material for: How to Understand Named Entities: Using Common Sense for News Captioning
Source: arXiv:2403.06520 source file (2024-03-11)
Supplement: Supplementary file 2 [file fig_context_vectors.tex]

\begin{figure*}
	\centering{\includegraphics[width=2.0\columnwidth]{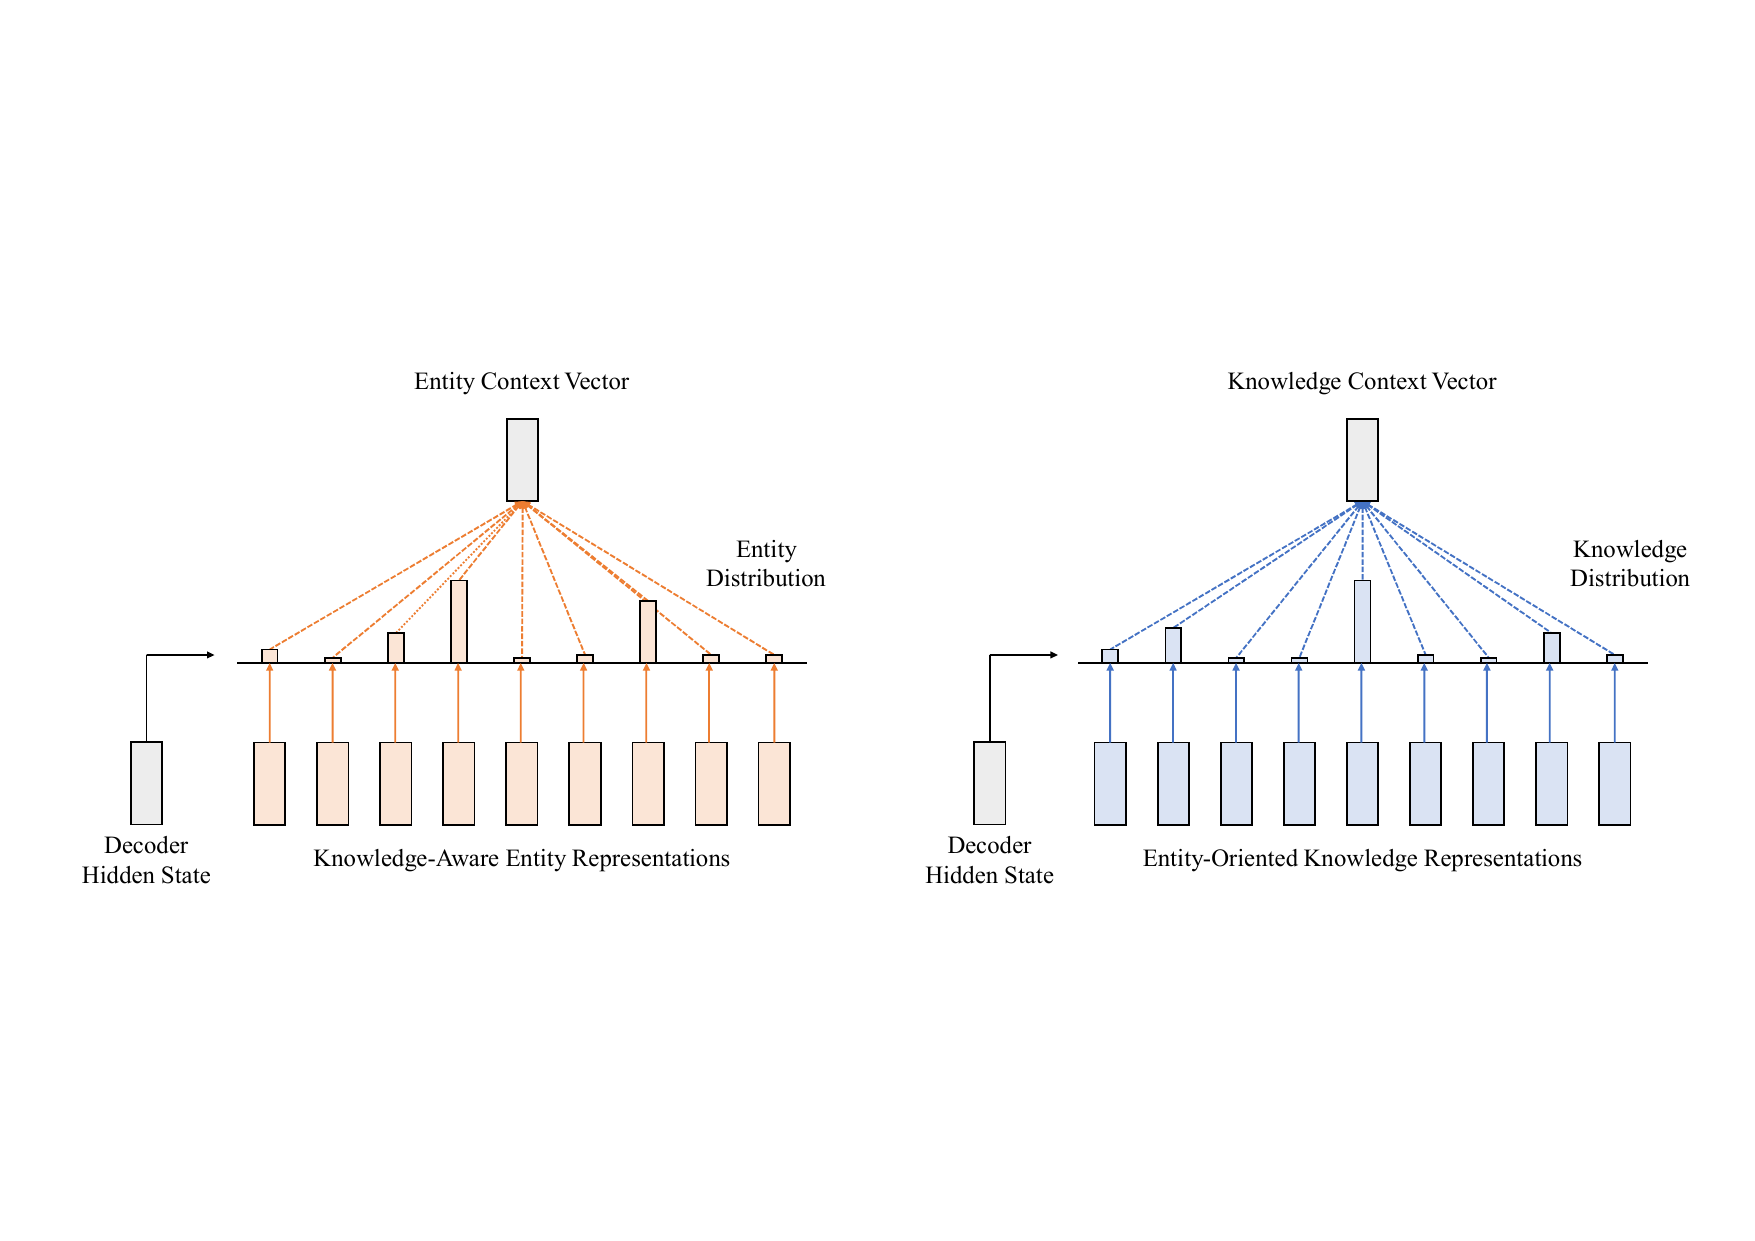}}
	\caption{Overview of the proposed method.
		(a) \textbf{Filter Module} aims to extract useful context and external knowledge of named entities for caption generation. 
		(b) \textbf{Distinguish Module} can distinguish similar named entities (e.g., ``Mr. Gates" and ``Mr. Sarkozy") by leveraging their semantic characteristics.
		(c) \textbf{Enrich Module} can associate weakly-related concepts of named entities to generate novel named entities (e.g., ``Bill Gates").
		(Best viewed in color)}
	\label{fig:framework}
%	\vspace{-0.4cm}
\end{figure*}
