# Supplementary material for: How to Understand Named Entities: Using Common Sense for News Captioning
Source: arXiv:2403.06520 source file (2024-03-11)
Supplement: Supplementary file 3 [file tab_entity_performance.tex]

\begin{table*}[!t]
	\centering
	\scalebox{1.0}{
		\begin{tabular}{ll|cccccccc}
			\toprule
			& \multirow{2}{*} {Model} 
			& \multicolumn{2}{c}{PERSON} 
			& \multicolumn{2}{c}{GPE} 
			& \multicolumn{2}{c}{ORG}   
			& \multicolumn{2}{c}{DATE} \\
			& & P & R & P & R & P & R & P & R \\
			\midrule
			
			\multirow{6}{*}{\rotatebox[origin=c]{90}{GoodNews}}
			& Non-Commonsense (Weighted Roberta)		& 27.96 & 22.89 & 24.79 & 24.85	& 22.07 & 19.69 & 14.53 & 12.92 \\
			& Non-Distinguish-Module (Weighted Roberta)	& 28.73 & 23.22 & 24.91 & 24.54	& 22.31 & 20.19 & 14.95 & 13.82 \\
			& Non-Enrich-Module (Weighted Roberta)		& 28.54 & 23.11 & 25.43 & 24.49	& 22.51 & 20.01 & 14.72 & 13.65 \\
			& Ours (Weighted Roberta) 
			& \textbf{28.48} & \textbf{23.12} & \textbf{24.79} & \textbf{24.71}	
			& \textbf{22.63} & \textbf{20.02} & \textbf{14.84} & \textbf{13.57} \\ 
			\cmidrule{2-10} 
			
			& Non-Commonsense (Full Model) 				& 29.50 & 23.32 & 25.40 & 25.19	& 22.36 & 20.22 & 15.18 & 13.57 \\
			& Non-Distinguish-Module (Full Model)		&		&		&		&		&		&		&		&		\\
			& Non-Enrich-Module	(Full Model)			& 29.57 & 23.91 & 25.82 & 25.78	& 22.39 & 20.45 & 15.15 & 13.79 \\
			& Ours (Full Model) 
			& \textbf{29.50} & \textbf{23.97} & \textbf{25.58} & \textbf{25.30}	
			& \textbf{22.26} & \textbf{20.49} & \textbf{14.90} & \textbf{13.54} \\    
			\midrule
			\multirow{3}{*}{\rotatebox[origin=c]{90}{NYTimes}}
			& Non-Commonsense (Full Model) 				& 36.96 & 31.28 & 26.70 & 31.08	& 21.56 & 18.71 & 14.42 & 14.30 \\
			& Non-Distinguish-Module (Full Model)		&		&		&		&		&		&		&		&		\\
			& Non-Enrich-Module	(Full Model)			& 38.28 & 32.59 & 27.18 & 31.06	& 21.92 & 18.60 & 14.74 & 14.53 \\
			& Ours (Full Model) 
			& \textbf{37.28} & \textbf{30.96} & \textbf{26.49} & \textbf{29.60}	
			& \textbf{20.85} & \textbf{18.33} & \textbf{14.72} & \textbf{13.79} \\

			\bottomrule
	\end{tabular}}
	\caption{Named entity generation performances (Precision and Recall) on several entity categories.}
	\label{tab:entity_performance}
	\vspace{-0.5cm}
\end{table*}
